# Supplementary material for: Deep Learning-Based Sparse Whole-Slide Image Analysis for the Diagnosis of Gastric Intestinal Metaplasia
Source: arXiv:2201.01449 source file (2022-01-05)
Supplement: Supplementary file 1 [file appendix.tex]

\appendix
I'm not sure whether to put derivations here or in Supplementary Material.
